# Supplementary material for: Acceleration via Symplectic Discretization of High-Resolution Differential Equations
Source: arXiv:1902.03694 source file (2019-11-04)
Supplement: Supplementary file 1 [file proof_c.tex]

\subsection{Technical Analysis of Subsection~\ref{subsec: low_c}}
\label{subsec: proof_low_c}

%%%%%%%%%%%%%%%%%%%%%%%%%%%%%%%%%%%%%%%%%%%%%%%%%%%%%%%%%%%%%%
\paragraph{Technical Analysis of Implicit Scheme~\eqref{eqn: low_NAG-C_im}}

The Lyapunov function is constructed as 
\[
\mathcal{E}(k) = (k + 1)(k + 2) s \left( f(x_{k}) - f(x^\star) \right) + \frac{1}{2} \left\| 2(x_{k} - x^\star) + (k + 1) \sqrt{s} v_{k} \right\|^{2}.
\]
%\[(k + 4) v_{k + 1} - (k + 1) v_{k} = - (k + 1) \sqrt{s} \nabla f(x_{k + 1})\]
Then the iterate difference can be calculated as
\begin{align*}
        \mathcal{E}(k + 1) - \mathcal{E}(k) 
 =      &               (k + 1)(k + 2) s \left( f(x_{k + 1}) - f(x_{k}) \right)  + 2(k + 2) s \left( f(x_{k + 1}) - f(x^\star) \right) \\
         & +            \frac{1}{2}\left\langle 2(x_{k + 1} - x_{k}) + (k + 2)\sqrt{s} v_{k + 1} - (k + 1) \sqrt{s} v_{k},\right. \\
         & \qquad\; \left. 2(x_{k + 1} + x_{k} - 2x^\star) + (k + 2) \sqrt{s} v_{k + 1} + (k + 1) \sqrt{s} v_{k}    \right\rangle \\
=       &               (k + 1)(k + 2) s \left( f(x_{k + 1}) - f(x_{k}) \right)  + 2(k + 2) s \left( f(x_{k + 1}) - f(x^\star) \right) \\
         &  -            \left\langle (k + 1) s \nabla f(x_{k + 1}),  2(x_{k + 1}  - x^\star) + (k + 2) \sqrt{s} v_{k + 1}  \right\rangle \\
         &  -            \frac{1}{2} (k + 1)^2 s^2 \left\| \nabla f(x_{k + 1}) \right\|^2. 
\end{align*}
Now, we hope to utilize the basic inequality for $f \in \mathcal{F}_{L}^{1}(\mathbb{R}^n)$ to make the right side of equality no more than zero. Based on the following inequalities:
\[
\left\{ \begin{aligned} 
         & f(x_{k + 1}) - f(x_{k})   \leq   \left\langle \nabla f(x_{k + 1}), x_{k + 1} - x_{k}    \right\rangle \\
         & f(x_{k + 1}) - f(x^\star) \leq  \left\langle  \nabla f(x_{k + 1}), x_{k + 1} - x^\star \right\rangle - \frac{1}{2L} \left\| \nabla f(x_{k + 1}) \right\|^{2},
         \end{aligned} \right.
\]
we can obtain
\[
\mathcal{E}(k + 1) - \mathcal{E}(k) \leq 2s \left( f(x_{k + 1}) - f(x^\star) \right) - \frac{(k + 1)s}{L} \left\| \nabla f(x_{k + 1}) \right\|^{2} - \frac{1}{2} (k + 1) s^{2} \left\| \nabla f(x_{k + 1})\right\|^{2}.
\]
Although the negative term contains the multiplier $k$ and $k^2$, we cannot guarantee 
that the right-hand-side is nonpositive.

% \leq   &  -            \frac{(k +1 )s}{L} \left\| \nabla f(x_{k + 1}) \right\|^{2}   - \frac{1}{2} (k + 1)^2 s^2 \left\| \nabla f(x_{k + 1}) \right\|^2 

%%%%%%%%%%%%%%%%%%%%%%%%%%%%%%%%%%%%%%%%%%%%%%%%%%%%%%%%%%%%%%%%
\paragraph{Technical Analysis of Explicit Scheme~\eqref{eqn: low_NAG-C_ex}}

The Lyapunov function is constructed as 
\[
\mathcal{E}(k) = (k - 2)(k - 1) s \left( f(x_{k}) - f(x^\star) \right) + \frac{1}{2} \left\| 2(x_{k} - x^\star) + (k - 1) \sqrt{s} v_{k} \right\|^{2}.
\]
We calculate the iterate difference
\begin{align*}
        \mathcal{E}(k + 1) - \mathcal{E}(k) 
 =      & (k - 1)k s \left( f(x_{k + 1}) - f(x_{k}) \right)  + 2 (k - 1) s \left( f(x_{k}) - f(x^\star) \right) \\
         & + \frac{1}{2}\left\langle 2(x_{k + 1} - x_{k}) + k \sqrt{s} v_{k + 1} - (k - 1)\sqrt{s} v_{k},\right. \\
         & \qquad\; \left. 2(x_{k + 1} + x_{k} - 2x^\star) + k \sqrt{s} v_{k + 1} + (k - 1)\sqrt{s} v_{k}    \right\rangle \\
=       &  (k - 1)k s \left( f(x_{k + 1}) - f(x_{k}) \right)  + 2 (k - 1) s \left( f(x_{k}) - f(x^\star) \right) \\
         & + \left\langle - k s \nabla f(x_{k}),  2(x_{k}  - x^\star) + (k - 1) \sqrt{s} v_{k }  \right\rangle  + \frac{1}{2} k^2 s^2 \left\| \nabla f(x_{k}) \right\|^2  
\end{align*}
\begin{itemize}
\item If we take the following basic inequality for $f \in \mathcal{F}_{L}^{1}(\mathbb{R}^n)$
\[
\left\{ \begin{aligned} 
         & f(x_{k + 1}) - f(x_{k})   \leq   \left\langle \nabla f(x_{k}), x_{k + 1} - x_{k}    \right\rangle + \frac{L}{2} \left\| x_{k + 1} - x_{k} \right\|^{2} \\
         & f(x_{k }) - f(x^\star) \leq  \left\langle  \nabla f(x_{k }), x_{k } - x^\star \right\rangle - \frac{1}{2L} \left\| \nabla f(x_{k }) \right\|^{2},
         \end{aligned} \right.
\]
we can obtain the following estimate
\[
\mathcal{E}(k + 1) - \mathcal{E}(k) \leq \frac{k(k - 1)Ls}{2} \left\| x_{k + 1} - x_{k} \right\|^{2} - 2s \left( f(x_{k}) - f(x^\star) \right) - \frac{ks}{L} \left\| \nabla f(x_{k}) \right\|^{2}+ \frac{k^2 s^2}{2} \left\| \nabla f(x_{k}) \right\|^{2},
\]
which cannot guarantee the right side of the inequality non-positive.

\item If we take the following basic inequality for $f \in \mathcal{F}_{L}^{1}(\mathbb{R}^n)$
\[
\left\{ \begin{aligned} 
         & f(x_{k + 1}) - f(x_{k})   \leq   \left\langle \nabla f(x_{k + 1}), x_{k + 1} - x_{k}    \right\rangle - \frac{1}{2L} \left\| \nabla f(x_{k + 1}) - \nabla f(x_{k}) \right\|^{2} \\
         & f(x_{k }) - f(x^\star) \leq  \left\langle  \nabla f(x_{k }), x_{k } - x^\star \right\rangle - \frac{1}{2L} \left\| \nabla f(x_{k }) \right\|^{2},
         \end{aligned} \right.
\]
we can obtain the following estimate
\begin{align*}
\mathcal{E}(k + 1) - \mathcal{E}(k) \leq & (k - 1) k s \left( \left\langle \nabla f(x_{k + 1}) - \nabla f(x_{k}), x_{k + 1} - x_{k} \right\rangle - \frac{1}{2L} \left\| \nabla f(x_{k + 1}) - \nabla f(x_{k}) \right\|^{2} \right) \\
                                                               &  2s \left( f(x_{k}) - f(x^\star) \right) - \frac{ks}{L} \left\| \nabla f(x_{k}) \right\|^{2}+ \frac{k^2 s^2}{2} \left\| \nabla f(x_{k}) \right\|^{2},
\end{align*}
which cannot still guarantee the right side of the inequality non-positive.
\end{itemize}

%%\[(k + 4) v_{k + 1} - (k + 1) v_{k} = - (k + 1) \sqrt{s} \nabla f(x_{k + 1})\]
%\[
%k v_{k + 1} - (k - 3)v_{k} = - k \sqrt{s} \nabla f(x_{k})
%\]

%%%%%%%%%%%%%%%%%%%%%%%%%%%%%%%%%%%%%%%%%%%%%%%%%%%%%%%%%%%%%%%%
\paragraph{Technical Analysis of Symplectic Scheme~\eqref{eqn: low_NAG-C_sym}}

The Lyapunov function is constructed as 
\[
\mathcal{E}(k) = (k + 1)^2 s \left( f(x_{k}) - f(x^\star) \right) + \frac{1}{2} \left\| 2(x_{k + 1} - x^\star) + (k + 1) \sqrt{s} v_{k} \right\|^{2}.
\]
Then the iterate difference is calculated as
\begin{align*}
        \mathcal{E}(k + 1) - \mathcal{E}(k) 
 =    & (k + 1)^2 s \left( f(x_{k + 1}) - f(x_{k}) \right)  + (2k + 3) s \left( f(x_{k + 1}) - f(x^\star) \right) \\
       & + \frac{1}{2}\left\langle 2(x_{k + 1} - x_{k}) + (k + 2)\sqrt{s} v_{k + 1} - (k + 1)\sqrt{s} v_{k},\right. \\
       & \qquad\; \left. 2(x_{k + 1} + x_{k} - 2x^\star) + (k + 2) \sqrt{s} v_{k + 1} + (k + 1)\sqrt{s} v_{k}    \right\rangle \\
=     &  (k + 1)^{2} s \left( f(x_{k + 1}) - f(x_{k}) \right)  + (2k + 3) s \left( f(x_{k + 1}) - f(x^\star) \right) \\
       &  - \left\langle (k + 1)s \nabla f(x_{k + 1}),  2(x_{k + 2}  - x^\star) + (k + 2) \sqrt{s} v_{k + 1}  \right\rangle \\
       &  - \frac{1}{2} (k + 1)^2 s^{2} \left\| \nabla f(x_{k + 1}) \right\|^2 
\end{align*}
Apparently, we hope to utilize the basic inequality for $f \in \mathcal{F}_{L}^{1}(\mathbb{R}^n)$ to make the right side of equality no more than zero. Taking the following inequalities 
\[
\left\{ \begin{aligned} 
         & f(x_{k + 1}) - f(x_{k})   \leq   \left\langle \nabla f(x_{k + 1}), x_{k + 1} - x_{k}    \right\rangle - \frac{1}{2L} \left\| \nabla f(x_{k + 1}) - \nabla f(x_{k}) \right\|^{2} \\
         & f(x_{k + 1}) - f(x^\star) \leq  \left\langle  \nabla f(x_{k + 1}), x_{k + 1} - x^\star \right\rangle - \frac{1}{2L} \left\| \nabla f(x_{k + 1}) \right\|^{2},
         \end{aligned} \right.
\]
we can obtain the following estimate
\[
\mathcal{E}(k + 1) - \mathcal{E}(k) \leq \frac{1}{2} (k + 1)^{2} s^{2} \left\| \nabla f(x_{k + 1}) \right\|^2 + s \left( f(x_{k + 1}) - f(x^\star) \right) - \frac{(k + 1)s}{L} \left\| \nabla f(x_{k + 1}) \right\|^{2},
\]
which cannot guarantee the right side of the inequality non-positive.

%\[
%(k + 4) v_{k + 1} - (k + 1) v_{k} = - (k + 1) \sqrt{s} \nabla f(x_{k + 1})
%\]
