# Supplementary material for: Acceleration via Symplectic Discretization of High-Resolution Differential Equations
Source: arXiv:1902.03694 source file (2019-11-04)
Supplement: Supplementary file 3 [file grad_norm.tex]

\begin{proof}[Proof of Theorem~\ref{thm: grad_descent_convex2}]
We consider the following Lyapunov function
	\[
	\mathcal{E}(k) = ks \left( f(x_{k}) - f(x^{\star}) \right) + \frac{1}{2} \left\| x_{k} - x^{\star}   \right\|^{2}.
	\]
We remark that this is just the discrete version of the Lyapunov function constructed by \citet{su2016differential}. The difference of this Lyapunov function satisfies
	\begin{align*}
	\lefteqn{\mathcal{E}(k + 1) - \mathcal{E}(k)}  \\
	& =       s \left( f(x_{k }) - f(x^{\star}) \right) + (k + 1) s  \left( f(x_{k + 1}) - f(x_{k}) \right) +  \frac{1}{2}\left\langle x_{k + 1} - x_{k}, x_{k + 1} + x_{k} - 2x^{\star} \right\rangle          \\
	&  \leq    s \left( f(x_{k }) - f(x^{\star})  -  \left\langle \nabla f(x_{k}), x_{k} - x^{\star} \right\rangle \right)  + (k + 1)s\left\langle \nabla f(x_{k}), x_{k+1} - x_{k} \right\rangle \\
	& \quad + \left[ \frac{(k + 1) s L}{2} + \frac{1}{2}\right]\left\| x_{k + 1} - x_{k}\right\|^{2} \\
	&  \leq    s^{2} \left[ - \frac{1}{2Ls} - (k + 1) +  \frac{(k + 1) s L}{2} + \frac{1}{2}  \right] \left\| \nabla f(x_{k}) \right\|^{2} \\
	&  \leq    - \frac{s^{2}}{2}  \left( k + 1 \right)  \left\| \nabla f(x_{k}) \right\|^{2}. 
	\end{align*}
Summing over $k$ and plugging in $s = 1/L$, we complete the proof.
\end{proof}
